# Supplementary material for: Positive Unlabeled Contrastive Learning
Source: arXiv:2206.01206 source file (2024-03-28)
Supplement: Supplementary file 1 [file appendix.tex]

\section{\textsc{PUCon} under non PU settings}
\label{sec:app.reduction}

\section{Background on Mixture Proportion Estimation}
\section{Additional Experimental Details}
\subsection{Model Architecture Details}
\lstset{style=mystyle}
\begin{lstlisting}[language=python]
def weights_init(m):
    if isinstance(m, (nn.Conv2d, nn.Linear)):
        nn.init.kaiming_normal_(m.weight)
        if m.bias is not None:
            nn.init.constant_(m.bias, 0.0)
\end{lstlisting}
\begin{lstlisting}[language=python]
class MLPContrastive(nn.Module):
    def __init__(self, nc, nh, hw, feat_dim=300, seed=1):
        super(MLPContrastive, self).__init__()
        torch.manual_seed(seed)

        layers = []
        sizes = [nc * nh * hw, 300, 300, 300, 300]
        layers.append(nn.Linear(sizes[0], sizes[1], bias=True))
        layers.append(nn.BatchNorm1d(sizes[1]))
        layers.append(nn.ReLU(inplace=True))

        layers.append(nn.Linear(sizes[1], sizes[2], bias=True))
        layers.append(nn.BatchNorm1d(sizes[2]))
        layers.append(nn.ReLU(inplace=True))

        layers.append(nn.Linear(sizes[2], sizes[3], bias=True))
        layers.append(nn.BatchNorm1d(sizes[3]))
        layers.append(nn.ReLU(inplace=True))

        layers.append(nn.Linear(sizes[3], sizes[4], bias=True))
        layers.append(nn.BatchNorm1d(sizes[4]))
        layers.append(nn.ReLU(inplace=True))

        self.backbone = nn.Sequential(*layers)

        self.projector = nn.Sequential(
            nn.Linear(sizes[4], 300, bias=True),
            nn.BatchNorm1d(300),
            nn.ReLU(inplace=True),
            nn.Linear(300, feat_dim, bias=True))

        self.online_head = nn.Linear(sizes[4], 1)
        self.apply(weights_init)

    def forward(self, x, mode='encode'):
        flatten_dim = 1
        for ix in range(1, len(x.shape)):
            flatten_dim *= x.shape[ix]
        x = x.reshape(x.shape[0], flatten_dim)

        if mode == 'encode':
            r = self.backbone(x)
            z = self.projector(r)
            return z

        elif mode == 'finetune':
            r = self.backbone(x)
            # r = self.testing(x)
            z = self.online_head(r)
            return z

        elif mode == 'feat_ext':
            r = self.backbone(x)
            return r

        else:
            raise NotImplementedError
-----------------
Num of Params = 637330
\end{lstlisting}

\begin{lstlisting}[language=python]
class CNNContrastive(nn.Module):
    def __init__(self, nc=3, feat_dim=1000, seed=1):
        super(CNNContrastive, self).__init__()
        torch.manual_seed(seed)

        # noinspection PyListCreation
        layers = []
        layers.append(nn.Conv2d(nc, 96, kernel_size=3, padding=1))
        layers.append(nn.BatchNorm2d(96))
        layers.append(nn.ReLU(inplace=True))

        layers.append(nn.Conv2d(96, 96, kernel_size=3, padding=1))
        layers.append(nn.BatchNorm2d(96))
        layers.append(nn.ReLU(inplace=True))

        layers.append(nn.Conv2d(96, 96, kernel_size=3, stride=2, padding=1))
        layers.append(nn.BatchNorm2d(96))
        layers.append(nn.ReLU(inplace=True))

        layers.append(nn.Conv2d(96, 192, kernel_size=3, padding=1))
        layers.append(nn.BatchNorm2d(192))
        layers.append(nn.ReLU(inplace=True))

        layers.append(nn.Conv2d(192, 192, kernel_size=3, padding=1))
        layers.append(nn.BatchNorm2d(192))
        layers.append(nn.ReLU(inplace=True))

        layers.append(nn.Conv2d(192, 192, kernel_size=3, stride=2, padding=1))
        layers.append(nn.BatchNorm2d(192))
        layers.append(nn.ReLU(inplace=True))

        layers.append(nn.Conv2d(192, 192, kernel_size=3, padding=1))
        layers.append(nn.BatchNorm2d(192))
        layers.append(nn.ReLU(inplace=True))

        layers.append(nn.Conv2d(192, 192, kernel_size=1))
        layers.append(nn.BatchNorm2d(192))
        layers.append(nn.ReLU(inplace=True))

        layers.append(nn.Conv2d(192, 10, kernel_size=1))
        layers.append(nn.BatchNorm2d(10))
        layers.append(nn.ReLU(inplace=True))

        self.backbone_cnn = nn.Sequential(*layers)

        self.backbone_lin = nn.Sequential(
            nn.Linear(640, 1000),
            nn.ReLU(inplace=True),
            nn.Linear(1000, feat_dim),
            nn.ReLU(inplace=True)
        )

        self.projector = nn.Sequential(
            nn.Linear(feat_dim, 1000, bias=True),
            nn.BatchNorm1d(1000),
            nn.ReLU(inplace=True),
            nn.Linear(1000, feat_dim, bias=True))

        self.online_head = nn.Linear(feat_dim, 1)

        self.apply(weights_init)

    def forward(self, x, mode='encode'):
        
        if mode == 'encode':
            r = self.backbone_cnn(x)
            r = r.view(-1, 640)
            r = self.backbone_lin(r)
            z = self.projector(r)
            return z

        elif mode == 'finetune':
            r = self.backbone_cnn(x)
            r = r.view(-1, 640)
            r = self.backbone_lin(r)
            z = self.online_head(r)
            return z

        elif mode == 'feat_ext':
            r = self.backbone_cnn(x)
            r = r.view(-1, 640)
            r = self.backbone_lin(r)
            return r

        else:
            raise NotImplementedError
------------------
Num of Params = 5019255
\end{lstlisting}
